# Supplementary material for: "Why wouldn't someone think of democracy as a target?": Security practices & challenges of people involved with U.S. political campaigns
Source: arXiv:2106.00236 source file (2021-06-01)
Supplement: Supplementary file 1 [file 09appendix.tex]

\section*{Appendix A: Script for Semi-Structured Interview}

\small
Thanks for taking the time to talk with us today! We will be going over a range of questions around security \& privacy, mostly as it relates to your role with and knowledge of [[                      ]]. If at any point you need to pause or to take a break, please let us know.

As we go through the questions, please keep in mind that this is not an evaluation of you or your experiences. For the purposes of this interview, there are no right or wrong answers -- we are here to learn from you and to understand your experiences and perspectives. Additionally, please be open and honest in what you share with us. If there's something you're uncomfortable sharing with us, we ask that you either tell us so or simply don't mention it rather than tell us something inaccurate. We're also open to hearing critical feedback.

Do you have any questions for us before we begin?

We'll turn on the audio recorder now.

\begin{enumerate}
    \item Can you give us a brief overview of your experiences with political campaigns?
\begin{itemize}
    \item What are/were your major responsibilities?
    \item How many people (approximately) are on the staff at [[ ]]?
    \begin{itemize}
        \item How many people are on the security team at [[ ]]?
    \end{itemize}
    \item Regarding one of the recent campaigns you've worked on, how many people were on the campaign staff?
    \begin{itemize}
        \item How many people were on the security team? IT staff?
        \item < if not known/mentioned > What was your role on that campaign?
    \end{itemize}
    \item What roles on that campaign did you most frequently interact with?
    \item < if applicable > Can you give us a brief description of your background in computer security or IT?
\end{itemize}
Thanks! Now let's move on to several questions around security and privacy as they relate to the political campaign(s) [[ you're part of / been on / support / you've supported ]].

\item What do you believe are the digital privacy- or security-related threats that political campaigns face?
\begin{itemize}
    \item Who would do this?
    \item Tell me more about why this attack / threat / risk matters
    \item How likely do you think this is to happen?
    \item What could be [[compromised / attacked / gained]]?
    \begin{itemize}
        \item What outcome are you worried about?
        \item Which data is at risk?
        \item Where is that data kept?
        \item Who has access to it?
      \end{itemize}
    \end{itemize}
    
\item Do you think the threats are any different for people involved in other types of campaigns? (e.g., what about the [[presidential ... senate … house of representative ... governor ... mayoral ... state senate ... school board ...]] races?)

\item Of course we don't want attacks like these to happen, so as Security and Privacy researchers, we look for weaknesses and vulnerabilities in systems and organizations
\begin{itemize}
    \item What are some areas that you worry about or think could be stronger in political campaigns?
    \item What role do you believe you have in helping prevent those things from happening?
    \item What role do you believe others play in helping prevent those things from happening?
\end{itemize}

\item What do you believe might get in the way of you doing your part in helping prevent those things from happening?

\item What do you believe might get in the way of others doing their part in helping prevent those things from happening?

\item < if unauthorized physical access not mentioned above >
What, if any, risks do you think there are to campaigns if someone were to gain unauthorized physical access to your/their offices?

\item What is the best security-related practice that people who work with political campaigns can do to protect their data and keep their people safe?
\begin{itemize}
    \item What is the security-related practice that you really wish they would do, but they just won't do it, or at least many of them won't do it?
    \begin{itemize}
        \item Why do you think they won't do it?
        \item Why do you think they should do it?
        \item What have you or others tried to do to get them to do it?
    \end{itemize}
\end{itemize}

\item When you need to communicate with the senior staff for a campaign, how do you do that?
\begin{itemize}
    \item How do you determine how you're going to communicate with them?
    \item Probes: Do they tell you / is it in a contract / do you try some things and see how responsive they are / Do you use whatever you normally use, and they just use that system?
    \item Is it different for the candidate?
\end{itemize}

\item Can you explain to us how emails, other communications, and doc access works (or worked) on the [[                 ]] campaign from above:
\begin{itemize}
    \item Who has email accounts on your [[G Suite / Microsoft 365]]?
    \begin{itemize}
        \item How many? 
        \item Did volunteers?
    \end{itemize} 
    \item Are there accounts for things like press@ or jobs@?
    \begin{itemize}
        \item Were these [[G Suite / Microsoft 365]] or separate <consumer email> accounts?
        \item How many people had access to those accounts?
        \item Where did you keep / distribute the passwords for those accounts?
        \item Did anyone ever change the passwords? Who? Why?
    \end{itemize} 
    \item Were you aware of any personal email accounts used for the campaign?
    \item What other accounts did you, the campaign, and the candidate have?
    \begin{itemize}
        \item Accounts to ad platforms/agencies
        \item Social media
        \item Voter files and other databases
        \item Web management
        \item Accounts with vendors/contractors
        \item Bank accounts
        \item Travel \& Reimbursement
        \item Calendars \& Scheduling
    \end{itemize} 
    \item How did you keep track of all of the accounts and their passwords?
    \item How many of the accounts do you think were closed / shutdown after the campaign ended?
\end{itemize}

We're now going to shift gears a little and talk about the security and privacy training that people involved in political campaigns may have had. We mean training quite broadly, from formal security courses to sitting in on a one-time 15 minute security demo or onboarding.

\item What, if any, security training have you taken as part of your work in politics? (probes: device policies, restrictions on apps, requirements or recommendations about advanced security features)
< if there are any of the above >
\begin{itemize}
    \item To whom does the training apply?
    \item Why was the training implemented?
    \item How are they taught?
    \item Who created them?
    \item What is working well?
    \item What isn't working well?
\end{itemize}

\item How likely do you believe that you, personally, are to be the target of phishing or hacking attempts, or attempts by others to access your digital accounts without your permission?
\begin{itemize}
    \item Who do you think would be targeting you?
    \item What do you think they would be after?
    \item Do you think the type of work you do has an influence on the phishing attempts you might receive?
\end{itemize}

Thanks! Our next set of questions focuses on authentication.

\item < if 2FA hasn't come up yet > Have you ever heard of 2-factor or multi-factor authentication?
\item < if yes or already mentioned > How would you describe 2FA to someone who works for a/the [[ ]] campaign?   
\begin{itemize}
    \item Probes:
    \begin{itemize}
    \item Tell me more about how you think that might help protect what's in your account?
    \item Why does [ getting a code texted to you ] protect your account more?
    \item Why is 2FA/MFA stronger protection for your account than a password?
    \item Why haven't you turned 2FA on for more of your accounts?
    \end{itemize}

\item < if correct or mostly correct > Right, and here are 6 we want to talk more about [[ handout ]]:

\item < if somewhere in between > Yes, and now we are going to look at 6 different types of 2FA, each of these are one additional method of proof that you are the person who should be able to log in to that account. And in this example, each of these would be used in combination with a password, so the two factors are the password paired with an item on the handout:

\item < if incorrect or mostly incorrect > Great, for the next activity we'd like everyone to use this definition of two-factor or multi-factor auth [[ go to < if no... > ]]

\item < if no, or if their explanation wasn't accurate > Multi-factor authentication is an authentication method that requires that you provide two or more types of evidence — usually a password and something else — to demonstrate that you're the legitimate account holder. For example, if one of your online accounts uses 2-factor authentication, you might have to sign in to that account with your password and a code that you receive via text message when you're trying to sign in to the account, or maybe your password and your fingerprint.
\end{itemize}

Those 6 are: < go to handout, also on next page >

\item Do you use or have you used multi-factor for any of your accounts?
\begin{itemize}
    \item < if yes > For which?
    \item Why did you start using it?
    \item < if stopped using it > Why did you stop using it?
\end{itemize}

\item What, if any, downsides do you believe multi-factor authentication has?

\item If you were using text messaging as your second factor, what security attacks do you think that account might still be vulnerable to?
\begin{itemize}
    \item What if you were using a phone call as your second factor?
    \item An app generator?
    \item A hardware token?
    \item A security key fob?
\end{itemize}

\item When it comes to campaigns, who do you think should use multi-factor authentication?
    \begin{itemize}
        \item For which accounts?
        \item Which type of authentication? Why?
        \item Do you see any challenges with getting them to use it?
    \end{itemize}

\item When you think about the threats and attacks we've discussed today, how do you think they might affect the 2020 elections?
\item How do you think, in the long-term, these threats or attacks could change the future?
\item Is there anything else you would like to say that we haven't covered?
\item Do you have any questions for us?
\end{enumerate}
