# Supplementary material for: "Why wouldn't someone think of democracy as a target?": Security practices & challenges of people involved with U.S. political campaigns
Source: arXiv:2106.00236 ancillary file (2021-06-01)
Supplement: Supplementary file 2 [file appendix.pdf]

## Appendix A: Interview Script and 2FA Handout

# Script for Semi-Structured Interview

*Thanks for taking the time to talk with us today! We will be going over a range of questions around security & privacy, mostly as it relates to your role with and knowledge of [[ ]]. If at any point you need to pause or to take a break, please let us know.*

*As we go through the questions, please keep in mind that this is not an evaluation of you or your experiences. For the purposes of this interview, there are no right or wrong answers -- we are here to learn from you and to understand your experiences and perspectives. Additionally, please be open and honest in what you share with us. If there's something you're uncomfortable sharing with us, we ask that you either tell us so or simply don't mention it rather than tell us something inaccurate. We're also open to hearing critical feedback.*

*Do you have any questions for us before we begin?*

*We'll turn on the audio recorder now.*

1. Can you give us a brief overview of your experiences with political campaigns?
    - What are/were your major responsibilities?
    - How many people (approximately) are on the staff at ________________?
        - How many people are on the security team at _________________?
    - Regarding one of the recent campaigns you've worked on, how many people were on the campaign staff?
        - How many people were on the security team? IT staff?
        - < if not known/mentioned > What was your role on that campaign?
    - What roles on that campaign did you most frequently interact with?
    - < if applicable > Can you give us a brief description of your background in computer security or IT?

*Thanks! Now let's move on to several questions around security and privacy as they relate to the political campaign(s) [[ you're part of / been on / support / you've supported ]].*

2. What do you believe are the digital privacy- or security-related threats that political campaigns face?
    - Who would do this?

- Tell me more about why this attack / threat / risk matters
- How likely do you think this is to happen?
- What could be [[ compromised / attacked / gained ]]?
    - What outcome are you worried about?
    - Which data is at risk?
    - Where is that data kept?
    - Who has access to it?

3. Do you think the threats are any different for people involved in other types of campaigns? (e.g., what about the [[ presidential ... senate … house of representative ... governor ... mayoral ... state senate ... school board ... ]] races?)
4. Of course we don't want attacks like these to happen, so as Security and Privacy researchers, we look for weaknesses and vulnerabilities in systems and organizations
    - What are some areas that you worry about or think could be stronger in political campaigns?
    - What role do you believe *you have* in helping prevent those things from happening?
    - What role do you believe *others play* in helping prevent those things from happening?
5. What do you believe might get in the way of you doing your part in helping prevent those things from happening?
6. What do you believe might get in the way of others doing their part in helping prevent those things from happening?
7. < if unauthorized physical access not mentioned above >
   What, if any, risks do you think there are to campaigns if someone were to gain unauthorized physical access to your/their offices?
8. What is the best security-related practice that people who work with political campaigns can do to protect their data and keep their people safe?
    - What is the security-related practice that you really wish they would do, but they just won't do it, or at least many of them won't do it?
        - Why do you think they *won't* do it?

        - Why do you think they *should* do it?
        - What have you or others tried to do to get them to do it?

9. When you need to communicate with the senior staff for a campaign, how do you do that?
    - How do you determine how you're going to communicate with them?
        - Probes: Do they tell you / is it in a contract / do you try some things and see how responsive they are / Do you use whatever you normally use, and they just use that system?
    - Is it different for the candidate?
10. Can you explain to us how emails, other communications, and doc access works (or worked) on the [[ ]] campaign from above:
    - Who has email accounts on your [[ G Suite / Microsoft 365 ]]?
        - How many?
        - Did volunteers?
    - Are there accounts for things like press@ or jobs@?
        - Were these [[ G Suite / Microsoft 365 ]] or separate <consumer email> accounts?
        - How many people had access to those accounts?
        - Where did you keep / distribute the passwords for those accounts?
        - Did anyone ever change the passwords?
            1. Who? Why?
    - Were you aware of any personal email accounts used for the campaign?
    - What other accounts did you, the campaign, and the candidate have?
        - Accounts to ad platforms/agencies
        - Social media
        - Voter files and other databases
        - Web management

        - Accounts with vendors/contractors
        - Bank accounts
        - Travel & Reimbursement
        - Calendars & Scheduling
    - How did you keep track of all of the accounts and their passwords?
    - How many of the accounts do you think were closed / shutdown after the campaign ended?

*We're now going to shift gears a little and talk about the security and privacy training that people involved in political campaigns may have had. We mean training quite broadly, from formal security courses to sitting in on a one-time 15 minute security demo or onboarding.*

11. What, if any, security training have you taken as part of your work in politics? (probes: device policies, restrictions on apps, requirements or recommendations about advanced security features)

    < if there are any of the above >

    - To whom does the training apply?
    - Why was the training implemented?
    - How are they taught?
    - Who created them?
    - What is working well?
    - What isn't working well?
12. How likely do you believe that you, personally, are to be the target of phishing or hacking attempts, or attempts by others to access your digital accounts without your permission?
    - Who do you think would be targeting you?
    - What do you think they would be after?
    - Do you think the type of work you do has an influence on the phishing attempts you might receive?

*Thanks! Our next set of questions focuses on authentication.*

13. < if 2FA hasn't come up yet > Have you ever heard of 2-factor or multi-factor authentication?

14. < if yes or already mentioned > How would you describe 2FA to someone who works for a/the _________ campaign?

    Probes:

    - Tell me more about how you think that might help protect what's in your account?
    - Why does [ getting a code texted to you ] protect your account more?
    - Why is 2FA/MFA stronger protection for your account than a password?
    - Why haven't you turned 2FA on for more of your accounts?

- < if correct or mostly correct > *Right, and here are 6 we want to talk more about [[ handout ]]:*

  < if somewhere in between > *Yes, and now we are going to look at 6 different types of 2FA, each of these are one additional method of proof that you are the person who should be able to log in to that account. And in this example, each of these would be used in combination with a password, so the two factors are the password paired with an item on the handout:*

  < if incorrect or mostly incorrect > *Great, for the next activity we'd like everyone to use this definition of two-factor or multi-factor auth [[ go to < if no... > ]]*

- < if no, or if their explanation wasn't accurate > *Multi-factor authentication is an authentication method that requires that you provide two or more types of evidence — usually a password and something else — to demonstrate that you're the legitimate account holder. For example, if one of your online accounts uses 2-factor authentication, you might have to sign in to that account with your password and a code that you receive via text message when you're trying to sign in to the account, or maybe your password and your fingerprint.*

*Those 6 are:* *< go to handout, at end of script >*

15. Do you use or have you used multi-factor for any of your accounts?

- < if yes > For which?
- Why did you start using it?
- < if stopped using it > Why did you stop using it?

16. What, if any, downsides do you believe multi-factor authentication has?
17. If you were using text messaging as your second factor, what security attacks do you think that account might still be vulnerable to?
    - What if you were using a phone call as your second factor?
    - An app generator?
    - A hardware token?
    - A security key fob?
18. When it comes to campaigns, who do you think should use multi-factor authentication?
    - For which accounts?
    - Which type of authentication?
        - Why?
    - Do you see any challenges with getting them to use it?
19. When you think about the threats and attacks we've discussed today, how do you think they might affect the 2020 elections?
20. How do you think, in the long-term, these threats or attacks could change the future?
21. Is there anything else you would like to say that we haven't covered?
22. Do you have any questions for us?

## Text message

when you try to sign in to an account, you might receive a text message that contains a one-time use code that's only good for a limited amount of time that you need to provide

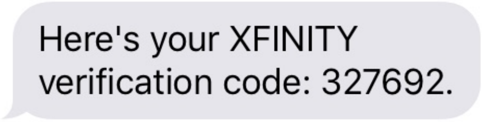


## Phone call

when you try to sign in to an account, you might receive a phone call with a one-time use code that's only good for a limited amount of time that you need to provide

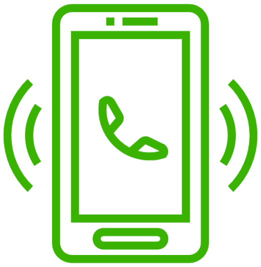

## App generator

when you try to sign in to an account, you might need to open an app on your phone that shows you a one-time use code that's only good for a limited amount of time that you need to provide

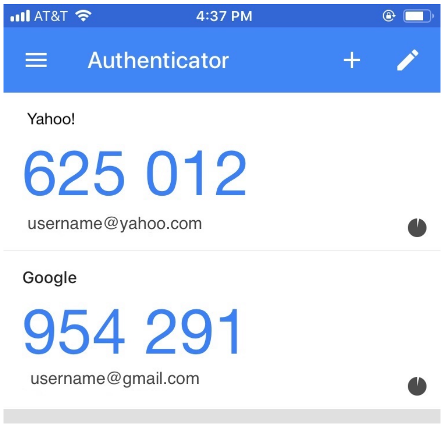


## Hardware token

when you try to sign in to an account, you might need to get your key fob-like device with a small digital screen that shows you a one-time use code that's only good for a limited amount of time that you need to provide

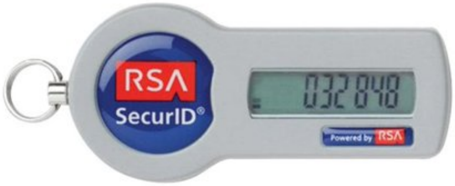


## Security key fob

when you try to sign in to an account, you might need to get your key fob-like device and either put it close to the device that you're trying to sign in to and push a button or insert it into the device you're trying to sign in to and tap it

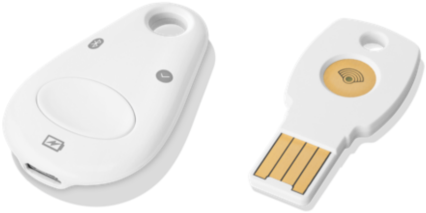

## Appendix B: Codes from Analysis

Below is the set of codes produced by applying the inductive coding procedures described in the Analysis section of this paper to our dataset, limited to the themes discussed in this paper. Note that these codes reflect *how participants talked about campaign security*; they are not intended to reflect a comprehensive technical categorization of security topics.

---

**(L1) Campaigns & closely related organizations:** An L1 (highest level) category of codes/data in our study. A characterization of campaigns and closely related organizations (party committees, consulting firms that support campaigns) that is relevant context for understanding data pertaining to our research goals and questions. The L2 & L3 codes below help focus coding on relevant context.

**(L2) Work culture:** A characterization of campaign work culture. Focus on the L3 codes below, which discuss characteristics of campaigns that appear to make prioritizing security hard.

**(L3) Goal: win election:** Statements or descriptions that the main goal of a campaign is to win the election.

**(L3) Temporary / Hard deadline:** Statements or descriptions of campaigns as temporary, transient, start ups with a quick ramp up, no existing institutional knowledge/infrastructure, or having a hard deadline (election day). This doesn't include mentions of people being too busy / not having enough time, which should be coded with the "Busy / Chaotic" code.

**(L3) Busy / Chaotic:** Statements or descriptions of campaigns as busy, hectic, disorganized, or chaotic. Also use this code for mentions of not having "time," feeling "pressure," being "intense," having "tight deadlines."

**(L3) Limited resources:** Statements or descriptions of campaigns as having limited resources. Resources could include money, equipment, or non-specific references to "resources." For time constraints, we use the "Busy / Chaotic" code, and for limited people resources/expertise, we use "Security knowledge is lacking."

**(L3) Amorphous boundaries:** Statements or descriptions of campaigns as having no clear lines between who is a campaign member (and thus needs to follow security policies, have managed accounts/devices, etc.) and who is not.

**(L3) General description:** General descriptions or other relevant characterizations of campaigns that help us understand contextual factors that might impact security, such as how many staff they employ, etc.

**(L2) Security culture:** A characterization of campaign security culture. Focus on the L3 codes below, which describe common ways campaign workers think about, behave regarding, or are positioned to address security.

**(L3) Security is a concern:** Statements or descriptions of people involved with campaigns being concerned about security. Could also include the participant saying they are concerned about security. This could be a broad statement, or a narrow statement about a particular security practice or threat.

**(L3) Security is not a concern:** Statements or descriptions of people involved with campaigns NOT being concerned about security. Could also include the participant saying they are not concerned about security. This could be a broad statement, or a narrow statement about a particular security practice or threat.

**(L3) Security is a priority:** Statements or descriptions of people involved with campaigns prioritizing security. Could also include the participant saying they personally prioritize security. This could be a broad statement about overall work culture, or a narrow statement about a particular decision in which they prioritized a more secure option.

**(L3) Security is not prioritized:** Statements or descriptions of people involved with campaigns NOT prioritizing security. Could also include the participant saying they personally did not prioritize security. This could be a broad

statement, or a narrow statement about a particular decision in which they didn't prioritize a more secure option.

**(L3) Security knowledge is lacking:** Statements or descriptions of campaigns lacking the knowledge to effectively assess, make decisions about, or implement security.

**(L3) General description:** General descriptions or other relevant characterizations of campaign security culture, including general or high level discussions of security culture.

**(L2) Levels:** Characterizations of the size, visibility, or contested nature of the campaigns that are being referred to in the snippet.

**(L3) Large / High-profile:** Presidential campaigns, contested campaigns, or campaigns that have otherwise received national attention.

**(L3) Medium:** Senate campaigns, Gubernatorial campaigns, or campaigns that have otherwise received state-wide attention.

**(L3) Small / Low-profile:** House campaigns, down ballot campaigns, or campaigns that have otherwise received only local attention.

---

**(L1) Practices [of campaigns & related orgs]:** An L1 (highest level) category of codes/data in our study. Data about campaign security-related practices – including those practices that protect against security threats and those that create security vulnerabilities. 2FA was the only practice that was explicitly prompted in all interviews, though participants usually brought it up first.

**(L2) Type [of Practice or Vulnerability]:** Categories of practices/vulnerabilities that represent major themes in our data and/or important vulnerabilities that the community should pay attention to.

**(L3) 2FA:** Characterizations of two-factor authentication or multi-factor authentication by people involved with campaigns, including its use, understandings of it, opinions about it.

**(L3) Accounts:** Data about accounts, as used or perceived by people involved with campaigns.

**(L3) Communications:** Data about written communications (email, messaging/chat, SMS), as used or perceived by people involved with campaigns.

**(L3) Devices:** Data about devices (phones, laptops, desktop computers, IoT devices), as used or perceived by people involved with campaigns.

**(L3) Other practices:** Data about practices other than those categorized above, as used or perceived by people involved with campaigns.

**(L2) Protective practice:** Category of codes that describe protective security-related practices that people involved with campaigns do or should do; i.e., preventative security behaviors. Note that the "Status" column augments these codes, and could indicate, for example, that people don't do the behavior ("Not used"), or that the participant thinks this is a best practice but isn't commenting on whether or not people do it ("Best practice"), or that the participant is sharing their opinion of the practice ("Opinion"), etc. Keep in mind when analyzing the practice codes that even when a practice is adopted, the level of adoption is often mixed ("Under-used" code under "Status").
When non-use of a protective practice (which creates a vulnerability) is more commonly described, we add codes under "Vulnerabilities," rather than relying on the "Protective practice" + "Not used" combo of codes. But for rare cases, we do use this combo.

**(L3) [2nd factor] [2FA]:** Accompanies the “2FA” type code to describe the specific second factor(s) discussed. E.g., security key, text codes, app codes, phone call, phone prompt, security questions, etc. Exclude if 2FA is discussed without naming specific second factors.

**(L3) Data stored in cloud [Accounts]:** Discusses the behavior of storing any data in the cloud. Implies that a cloud service account is used, so tends to accompany the “Accounts” type code.

**(L3) Identify/avoid phishing/scams [Accounts]:** Discusses behaviors to identify and/or avoid phishing or scams. Because this is about account security, it tends to accompany the “Accounts” type code.

**(L3) Managed work accounts [Accounts]:** Discusses behaviors related to accounts where use can be limited and/or monitored. These can include enterprise suites or any software that allows any amount of limiting and monitoring. Often, coverage of all people and all accounts used by people involved in a campaign is not exhaustive – use this code for any level of adoption.

**(L3) Security alerts [Accounts]:** Discusses the behavior of seeing or turning on security alerts. Some security alerts are set by default without being turned on, and just remembering and noting that someone saw a security alert is sufficient to apply this code. Because this is about account security, it tends to accompany the “Accounts” type code.

**(L3) Good password practices [Accounts, Devices]:** Discusses good password-related behaviors (e.g., using a password manager, using long & unique passwords, etc.). Because this is usually about account or device security, it tends to accompany the “Accounts” or “Devices” type codes.

**(L3) Encryption [Accounts, Devices, Communications]:** Discusses encryption-related behaviors (e.g., using E2E encrypted messaging, encrypting device data, etc.). Because this is usually about the security of content within account or device security, and most often communications data, it tends to accompany the “Accounts” or “Devices” or “Communications” type codes.

**(L3) Avoid tech / Comm with care [Communications]:** Discusses the behaviors of avoiding technology (typically to keep sensitive information from being captured/stored digitally in the first place) or of “communicating with care” (i.e., self-censoring or choosing one’s words carefully when putting them in digital writing). This tends to accompany the “Communications” type code (although it could involve other documentation).

**(L3) Security rules / policies [Other]:** Discusses rules or policies for staff that campaigns, orgs, committees, etc. put in place to protect their security. E.g., enforced 2FA, data retention policies, etc.

**(L3) Security education [Other]:** Discusses training / education people attend or offer aimed to improve security awareness / knowledge. Includes a range from formative/lightweight (e.g., a presentation at a conference or an onboarding session for new campaign staff), to moderate levels (e.g., regular access to a security knowledgeable IT staff member), to more extensive training.

**(L3) Hire vendor / outsource security [Other]:** Discusses outsourcing security to a vendor, or the sentiment that hiring a vendor will address security needs for the campaign or organization.

**(L3) Share knowledge / info [Other]:** Discusses people (within or across organizations/industries) sharing knowledge or information related to security, as a way of raising awareness of new risks, breaches, best practices, etc., in order to prevent them. The goal is for people to band together against common attackers or threats.

**(L3) Secure file sharing [Other]:** Discusses file sharing in secure ways, such as via cloud provider ACLs, reviewing and updating old ACLs, avoiding email attachments, etc.

**(L2) Status [of Practice]:** These descriptors refer to the Practice code. Sometimes a Who code will be used, referring to who does or does not do the practice.

**(L3) Used:** The Practice is used, at least by most of the Who indicated.

**(L3) Not used / Under-used:** The Practice is not used, or is under-used by the Who indicated. "Under-used" also refers to mixed use, where a good number of people use the practice, but a notable number of others don't (e.g., "we can get all the staff to do this, but none of the consultants").

**(L3) Best practice / Recommended:** The Practice is a best practice or is recommended, either by the participant (most often) or someone else they are referring to.

**(L3) Explanation - [researcher assessment of explanation]:** The participant is explaining the Practice. This enables the researchers to assess how well the participant understands the practice (or at least how well they can explain it). When appropriate, include some notes assessing comprehension.

**(L3) Opinion:** The participant expresses an opinion (attitude, sentiment) about the Practice.

**(L2) Vulnerabilities:** Category of codes that describe practices, or qualities of the data or individuals involved, that appear to result in security vulnerabilities for campaigns. Note that the "Not used / Under-used" code overlaps with the "Vulnerabilities" codes (since not using a protective practice often creates a vulnerability) – we are double-coding to aid analysis. The vulnerabilities with [Accounts] are typically applicable to accounts, with [Devices] are typically applicable to devices, and so on.

**(L3) Tech mistakes / misunderstood tech [Any]:** Discusses a security-related practice or technology that represents a mistake in use or a misunderstanding of the technology or how to properly use it. This code may be referring to a Practice code.

**(L3) Shared account [Accounts]:** Discusses accounts that are used by multiple people, which usually meant accounts security practices were weaker (e.g., shared credentials, weaker passwords, no 2FA, etc.).

**(L3) Transiently owned account [Accounts]:** Discusses accounts for which ownership is passed from person to person with relative frequency/regularity. This usually meant accounts security practices were weaker (e.g., old owners retaining credentials, no 2FA, etc.).

**(L3) Too many accounts [Accounts]:** Discusses the practice of using lots of accounts, which increases the surface area for attackers and makes it harder for users (and admins) to ensure the strongest forms of protection for each account.

**(L3) Sensitive / targeted [data, individual] [Accounts, Communications, Other]:** Discusses the quality of data being sensitive (i.e., damaging if leaked or stolen) and/or data or individuals being targeted (i.e., a goal of attackers is to steal or leak). These are together because participants often describe data as being both sensitive and targeted, simultaneously.

**(L3) Personal [account/device] use [Accounts, Devices]:** Discusses the use of personal accounts or devices, for both work and personal content, by people involved with campaigns. Typically, personal accounts and devices cannot be managed/secured/monitored by IT staff or policies, and thus have weaker security protections. The personal content in these accounts/devices is as targeted as work content, since it can be used to embarrass the campaign.

**(L3) Poor password practices [Accounts, Devices]:** Discusses password practices that create security vulnerabilities, such as weak passwords, password reuse, sharing/storing passwords in insecure places, not using a

password manager, etc.

**(L3) Oversharing on social media or in comms [Other]:** Discusses social media or communications (email, chat) practices that result in sharing "too much" information with adversaries. One common case is purposefully sharing something on social media that others on the campaign are not ready to reveal or that is accidentally of use to adversaries, e.g., staffers who release sensitive info too early, or even who reveal they work for the campaign and thus become targets. Another example is ad hoc forwarding of sensitive emails beyond the original recipients.

**(L3) File ACLs / Oversharing [Other]:** Discusses poor use of data/file ACLs (access control lists / permissions), such as not setting them up securely, not removing people who should no longer have access, etc. A few cases coded with this code referred to data access more vaguely, and it was unclear if it was a file, an account, or some other format (e.g., "voter data" or "research book") – if the example was about oversharing data, then we used this code.

**(L3) Feels helpless [Other]:** Discusses the reaction of feeling helpless regarding security, which may result in them not taking preventative actions. Some of these may relate to "learned helplessness," a mental state in which users feel unable or unwilling to avoid security issues that are avoidable. Here, we code any mentions of helplessness, as it may lead to learned helplessness later.

**(L3) Do nothing / ignore [Other]:** Discusses ignoring or doing nothing in response to a vulnerability, risk, or attack.

---

**(L1) Who:** An L1 (highest level) category of codes/data in our study. Inferred or explicitly stated actor about which the snippet refers. These are often inferred by who the participant typically works with, or previous snippets that explicitly state an actor.

**(L2) Campaign Insiders:** These refer to actors inside the campaign or related organizations that support campaigns (i.e., within the "amorphous boundaries" of a campaign). These typically refer to who is being characterized by the Campaign and Practices codes above, or who is being targeted for attacks or by attackers.

**(L3) Candidate / Elected official:** The candidate around which the campaign centers, or an incumbent who is both an elected official and a candidate, or the candidate once elected.

**(L3) [Senior / Junior] Campaign staff / Campaigns:** Any references to campaign staff or "campaign(s)." Often, campaign staff was implied by the participant's context – that is, they work(ed) on/with campaigns and were speaking throughout the interview of those experiences. These implied cases are coded based on context from earlier in the interview. Participants also sometimes referred to the campaign(s) as an actor instead of any particular individual/group on the campaign. For example, "the campaign decided to use 2FA," "campaigns generally don't use these security precautions," "the campaign kept it's data in the cloud," etc. These cases were coded "Campaign staff," though we note that this is a fuzzy interpretation, but accurately reflects the general fuzziness of campaign boundaries, and fuzziness of how participants talked about actors on a campaign.
When specified, indicate if senior or junior staff are specifically mentioned as follows: - Senior staff: Campaign staff and consultants that form the main decision makers and central team working with the candidate. Often includes the campaign manager, finance director, media/digital director, communications director, field coordinator, direct mail person, and pollster/research. - Junior staff: Low level staff on a campaign, typically described as young, fresh out of college, and/or in their first job.
We note that participants typically lumped staff and consultants together when they talked about people working on campaigns. Consultants often made up the senior staff and core campaign experts, so were very embedded in the actions and work culture of a campaign. Thus this code must be interpreted with this in mind: many snippets coded with "Campaign staff" will incorporate consultants without saying so and without being coded "Consultant / Vendor." We do add the "Consultant / Vendor" code when participants are explicit, e.g., that a "Senior campaign staff" member is also a "Consultant."

**(L3) Consultant / Vendor:** Consultants work for multiple campaigns and are often more senior political experts. They can be decision makers on a campaign. Typically, they are self-employed or part of a small firm that has its own domain/email provider that is separate from the campaign's.
Vendors provide a particular service and/or toolset to multiple campaigns, such as IT, security, voter data, online fundraising, emailing, and so on.
Participants used these terms interchangeably, so we do not differentiate between them in the coding.

**(L3) Volunteer:** Volunteers work for the campaign but are not paid staff. They are inherently temporary workers, may come and go, may work only once or come back repeatedly. They are usually discussed as valuable assets to a campaign, but also sometimes as introducing security threats. Typically volunteers do not have campaign domain accounts, but some repeat volunteers in specific roles (e.g., organizing groups of other volunteers) may get domain accounts.

**(L3) Organization staff:** Staff at national or state party committees (e.g., DCCC, DNC, RNC, NRSC, etc.), or political organizations (e.g., PACs, think tanks, etc.) that support campaigns.

**(L3) Family & friends:** Family & friends of the candidate or other campaign members. These tended to include mentions of the candidate's family needing to set up security precautions, and the candidate's friends helping them set up or run aspects of the campaign. (We excluded mentions the participant made to their own family or friends, unless they were related to security on campaigns.)

**(L3) Self:** The participant referring to themselves (e.g., their own practices, attitudes, or understandings).

**(L2) External Actors (with respect to the campaign):** These refer to actors outside of the campaign or related organizations that support campaigns. Some of the actors below were (suspected of) carrying out an attack (listed further below). Other actors were discussed as having other types of important relationships. For attackers, we also coded when a participant explicitly stated a specific attacker was NOT a concern.

**(L3) Nation-states:** Agents of national governments; typically this referred to foreign (non-US) governments.

**(L3) Opponent:** Anyone who opposes the candidate in a race, whether it is an individual or group from the same or other political party. Note that this was the only way that participants referred to members of their own party as adversaries (e.g., during a primary, someone from your own party or even your party's committees could be seen as opponents). This code overlaps with other "external actor" codes; use this one when the participant discusses opponents in broader ways than the other codes.

**(L3) Other political party:** The opposing political party with respect to the campaign/orgs being discussed, including entities that may be seen to represent that party (e.g., the official national and state committees, individual campaigns, etc.). In the US two-party system, this was typically referring to actors from either the Republican or Democratic parties.

**(L3) Citizens:** Individual US citizens. We focused on cases when citizens were described as security threats or as adversaries, e.g., exhibiting "trolling," "crazy" or "attention seeking" behavior.

**(L3) Thieves:** People aiming to steal money or valuables from campaigns, with the apparent goal of profiting.

**(L3) Profiteers:** People leveraging *information campaigns* apparently to make money.

**(L3) Special interest group:** PACs or other organized groups perceived to have political agendas.

**(L3) Press:** Members of the press or media (e.g., reporters, bloggers, etc.).

**(L3) Anyone / Others:** Used for vague references to anyone or any others beyond who the participant had discussed (e.g., "anyone could be an attacker").

---

**(L1) Attacks & Harms:** An L1 (highest level) category of codes/data in our study. Data about campaign security-related attacks and their harms.

**(L2) Attack types:** Category of codes that describe security-related attacks that adversaries use on people involved with campaigns. We organize attacks into several high level L3 attacks that can be further broken down into somewhat more specific L4 attacks. Note that this organization is imperfect and non-standard from a security technology viewpoint; instead it reflects how participants talked about the attacks, as they applied to campaigns, in their experience.

**(L3) Phishing:** Discusses phishing attacks, which are fraudulent attempts to obtain sensitive information or data, such as usernames, passwords, or credit card details, by disguising oneself as a trustworthy entity in an electronic communication.
For the purposes of coding, we define "Impersonation / Social engineering" to be everything that isn't explicitly covered by the Phishing definition above. But there is still some gray area between "Phishing" and "Impersonation / Social engineering." We exclude phone calls from "Phishing" and instead code them "Impersonation / social engineering." We also exclude listening in on video calls or conference calls from "Phishing." When participants explicitly talk about "phishing" or "phish," but do not talk about the details of this type of attack, we use the "Phishing" code.

**(L3) Hacking / other remote attack:** Discusses attacks where an attacker "hacks" the target and/or leverages some presumably remote mechanism to compromise or otherwise harm the target's devices, accounts, data, or access. From non-security expert participants, these were often vague, as if the participant didn't know exactly what the attacker did. From more expert participants, these include discussions of the more sophisticated attacks nation-states can and allegedly have leveraged to target individuals on campaigns.

**(L4) Account compromise:** Discusses attacks where the attacker "hacks" the target to gain access to their accounts. If more specific codes are applied (e.g., phishing), we do not double-code with this code. This code tended to be used when participants communicated a more vague sense of how attackers gained access to the account.

**(L4) Device / system / network compromise:** Discusses attacks where a device, system, or network is compromised. Participants often used the terms "system" and "network" vaguely (e.g., it's possible the actual mechanism is an account compromise). If more specific codes are applied (e.g., malware), we do not double-code with this code.

**(L4) Zero-day / Unknown:** Discusses novel and / or unknown security attacks that are thus hard to protect against.

**(L4) DoS:** Discusses "denial of service" attacks where an attacker prevents people from accessing or making use of some digital resource.

**(L4) Malware / ransomware:** Discusses attacks where an attacker installs or tricks a target into installing malware or ransomware on a device or system. These were discussed as a type of "device compromise," but we do not double-code this item with that code. These were sometimes described as remote attacks and sometimes as physical attacks, but we categorize all instances here under "Hacking / other remote attacks."

**(L3) Physical attack:** Discusses attacks where an attacker uses physical access to devices, networks, office spaces, or individuals to gain access to campaign information. Requires the attacker to be physically proximate to a campaign office, worker, or place a worker frequents (like their home or gym).

**(L4) Walk into office:** Discusses attacks where an attacker physically walks into a campaign office to gain access to digital devices or systems.

**(L4) Stolen / seized device:** Discusses attacks where an attacker steals or seizes a device. Some of these were thefts unrelated to the campaign specifically.

**(L4) Recording:** Discusses attacks where an attacker is physically near the candidate or campaign workers, and video or audio records them. Then typically select, out-of-context recordings are released to the public to embarrass the candidate/campaign.

**(L4) USB / Plug-in:** Discusses attacks where a USB or other plug-in is leveraged to compromise a device.

**(L4) Violence:** Discusses attacks where someone is subject to threats of physical violence or actual physical violence.

**(L3) Impersonation / Social engineering (non-phishing):** Discusses attacks where an attacker poses as someone other than themselves or otherwise manipulates someone into giving the attacker information, money, or other valuables, using means that are not explicitly covered by the "Phishing" definition above. This includes in person, phone, or video conferencing approaches.
There is some gray area between "Phishing" and "Impersonation / Social engineering." For the purposes of coding, we exclude phone calls from "Phishing" and instead code them "Impersonation / social engineering," because phone calls are low-tech and existed as a vector of attack prior to the advent of electronic communication. We also include listening in on video calls or conference calls in "Impersonation / Social engineering," since the attacker did not initiate communication with the target in these cases and due to their similarity to phone call-based attacks. When participants explicitly talk about attackers "impersonating" or "social engineering" in the context of a phishing attack, but do not describe any interactions beyond those covered by the Phishing definition, we only code these snippets "Phishing."

**(L3) Opportunism:** Discusses attacks where an attacker takes advantage of someone who overshares (e.g., puts info that can be exploited on social media) or accidentally leaks information (e.g., talks about confidential info in a public space; loses their phone on the subway). These do not include cases when an attacker premeditates and put effort into their attack; instead, the opportunity falls in their lap.

**(L4) Other:** Any other explicitly mentioned type of toxic content, such as digital content depicting violence, radicalizing content, etc.

**(L3) Any:** Discusses security attacks, without specifying which one. For example, "I am worried about security attacks."

**(L2) Attack goals:** Category of codes that describe the perceived goal of attackers who use the security attacks above on people involved with campaigns, according to the participant. Some of these are explicitly stated, whereas others are implied. This category is about the direct outcomes of an attack, which ultimately can lead to "harms" experienced by campaigns and the U.S. as a whole (as described by the next L2 category).

**(L3) Confidential info leak:** Discusses cases when the attacker's goal is believed to be to leak confidential information pertaining to the campaign.

**(L3) Confidential info theft:** Discusses cases when the attacker's goal is believed to be to steal confidential information pertaining to the campaign.

**(L3) Monetary theft:** Discusses cases when the attacker's goal seems to be to steal money from the campaign.

**(L3) Inability to work:** Discusses cases when the attacker's goal seems to be to prevent people involved with the campaign from working. For example, preventing them from reaching voters by locking them out of voter databases, preventing them from fundraising by taking down their donation website, etc.

**(L3) Voters polarized / misinformed / influenced:** Discusses cases when the attacker's goal seems to be to misinform voters / Americans, and/or create discord among them, and/or to influence their opinions or votes.

**(L3) Coercion / control:** Discusses cases when the attacker's goal seems to be to control another individual or an entity, and coerce them into certain actions.

**(L2) Harms:** Category of codes that describe the resulting harm following a security-related attack. We organize attacks into two high level L3 harms that can be further broken down into somewhat more specific L4 harms.

**(L3) Election loss / outcomes changed:** Discusses the harm of losing an election that might otherwise have been won if it weren't for the attack. Apply this code for anything election loss related that isn't already covered by the L4 codes below, or when participants specifically say an election could be lost or changed as a result of an attack.

**(L4) Embarrassment / Bad PR:** Discusses the harm of voters seeing or being exposed to information that causes them to think less of a candidate, campaign, or party.

**(L4) Loss of strategic edge:** Discusses the harm of a campaign losing a potential advantage over their opponent.

**(L4) Monetary loss:** Discusses the harm of a campaign losing money they could have spent to win the election.

**(L4) Loss of voters:** Discusses the harm of a campaign losing voters who may have otherwise voted for their candidate.

**(L3) Democracy damaged:** Discusses harm to democracy in the U.S. as a result of a security attack.

**(L3) Other:** Discusses other or non-specific harms.

---

**(L1) Other:** An L1 (highest level) category of codes/data in our study. A category for a miscellaneous set of L2 & L3 codes that cover topics of interest to the research goals.

**(L2) Technology:** Data pertaining to technology design or specific areas of technology that are not covered above.

**(L3) Feature request:** Any technology feature request, or ask of the technology community.

**(L3) Pain point:** Description or statement of a problem with technology, such as a usability issue, a challenge using or understanding technology, mismatch between the technology and needs, etc.

**(L2) Example / story:** Includes a real-life example or story about the theme/codes applied.

**(L2) Good quote:** A researcher assessment of whether a quote may be high quality enough for inclusion in reports.

# Appendix C: Recruiting Material Example

**Security & Privacy in Government & Politics study**

We're contacting you to ask you to consider participating in an upcoming research study with Google. As you can probably tell by the study's name, the focus is on security and privacy in government and politics. Your input during studies such as this one helps to enhance the products and services we offer and make them work better *for everyone*.

We're currently scheduling participants for the first round of the study, which will take place in Washington, DC from <dates> at the Google DC office or we can come to you.

We thought you would be a great fit for this study, so we hope you'll consider participating. If you know you'd like to participate, or if you'd like to learn more, please contact the researchers at <email>.

If you'd like to learn more about the researchers (Sunny Consolvo, Patrick Gage Kelley, and Elie Bursztein), please see the <attached PDF>.

Thanks so much for considering it!

# **Appendix D: Consent Form** – not for reuse

## Google Data Collection Informed Consent

1. **Purpose.** We are pleased to invite you to participate in a user research study ("Study") conducted by Google LLC ("Google" or "We"). The purpose of the Study is to assist Google to design, research, develop, build, and improve its current and future products and services ("Purpose"). The study involves a product or feature that's currently in development; and will help the Google team better understand the needs of our users.

2. **Participation.** By participating in the Study you confirm: (a) you are over eighteen (18) years old; and (b) participating in the Study will not violate any agreement with a third party or create a conflict of interest. Your participation in this Study is completely voluntary. You may choose to withdraw at any time during the Study without any penalty. You may also decline to answer any particular question you do not wish to answer for any reason. The researchers also have the right to end the Study at any time.

3. **Incentives.** No incentive is being offered for your participation in this study.

4. **Audio/Video/Photography.** This study involves collecting audio, video, or photographs.

   a. **Risks.** We are not aware of any physical or emotional risks associated with participation in the Study. However, you may feel uncomfortable or embarrassed while being photographed or filmed.

   b. **Consent.** With your consent, we may capture your face, voice, physical features, mannerisms, likeness, and interactions through photography, screen recording, and audio/video recording during the Study session, for the Purpose. We may ask you to remotely share your device screen with the researchers to observe your interaction with the product or app.

   **I give my consent: ________**

5. **Study Data Use and Retention.** We may retain, use, or share Study data that does not personally identify you for any purpose and without limitation. We may retain your personal information in the Study data as long as it is necessary for the Purpose. Any personal information in the Study data that could identify you such as your name, email, video or demographic data may be shared internally for the Purpose.

6. **Personally Identifiable Information.** With your consent, we may collect and process personally identifiable information in accordance with this agreement and Google Privacy Policy at https://policies.google.com/privacy. For example, we may ask for your name, email address, phone number and other information that may identify you.

   **I give my consent: ________**

7. **Sensitive Personally Identifiable Information.** With your consent, we may collect and process sensitive personally identifiable information such as information pertaining to race, religion, sexual orientation, or health in accordance with this agreement and Google Privacy Policy at https://policies.google.com/privacy.

   **I give my consent: ________**

8. **Data Transfer.** You consent to Google processing Study data outside the country or region where the data is originally collected or where you are located, including in countries where you may have fewer rights in respect of your information than you do in your country of residence. Study data may be processed by Google in the United States or Google affiliates and service providers acting on Google's behalf outside of your country of residence.

9. **Data Storage and Protection.** We respect your privacy and use a variety of measures to protect your personal identifying information from unauthorized access and disclosure in accordance with Google Privacy Policy at https://policies.google.com/privacy.

10. **Sharing with Third Parties.** Google may want to share the Study data that personally identifies you with certain third parties such as Google affiliates and contractors who agree to meet our standards for protecting Study data and who have a need to access the Study data in furtherance of the Purpose.

11. **Google Confidential Information.** This agreement and any information provided to you by Google during the Study are confidential (the "Confidential Information"). You agree to (i) use Confidential Information only for participation in the Study, (ii) take reasonable degree of care to prevent any unauthorized use or disclosure of Confidential Information, and (iii) not photograph, record, or share any Confidential Information with anyone. Your duty to protect Google's Confidential Information expires five years from disclosure.

12. **Questions/Requests for Deletion.** If you have questions or wish to have your personal data contained in the Study data deleted, please email us at uxquestions@google.com. The subject of your email should be "User Experience Study Data Request" and your email should include enough information (location, date, time, etc) so that Google can identify the Study data collected from you (if applicable). Study data that contains or is linked to your personal information will be deleted as soon as reasonably practicable, unless otherwise prohibited by applicable legislation or legal process. Google may, in its sole discretion, retain Study data that does not personally identify you for a longer duration or for any future study.

13. **Feedback.** In the course of your participation in the Study, you may provide comments, feedback, ideas, reports, suggestions, data, or other information to Google relating to Google products and services (collectively "Feedback"). For clarity, Feedback is separate from and not part of the Study data. Google may use any Feedback without restriction to develop and improve Google's current or future products and services. You agree that you will not disclose to Google any third party information that you are otherwise obligated to maintain as confidential. Google has no obligation to use your Feedback.

14. **General Provisions.** Unless applicable law requires otherwise: (a) this agreement is governed by the laws of the State of California, excluding its conflictoflaws principles; and (b) the exclusive venue for any dispute relating to this agreement will be Santa Clara County, California. Any amendments must be in writing. Failure to enforce any of the provisions of this agreement will not constitute a waiver. This agreement does not create any agency or partnership relationship. If any term (or part of a term) of this agreement is invalid, illegal or unenforceable, the rest of the agreement will remain in effect. This section will survive any termination of this agreement. You can contact your local data protection authority if you have concerns regarding your rights under local law.

Agreed and accepted by:

Full Name: ______________________________

Signature: ______________________________

Email Address: ______________________________

Date: ______________________________
